# Supplementary material for: Expanding the Action Space of LLMs to Reason Beyond Language
Source: arXiv:2510.07581 source file (2025-10-17)
Supplement: Supplementary file 1 [file main_appendix_only.tex]

\documentclass{article} % For LaTeX2e
\usepackage{iclr2026_conference,times}

% Optional math commands from https://github.com/goodfeli/dlbook_notation.
\input{math_commands.tex}

\usepackage{hyperref}
\usepackage[nameinlink]{cleveref}
\usepackage{url}
\usepackage{tikz}
\usepackage[edges]{forest}
\usepackage{multirow}
\usepackage{booktabs}
\usepackage{fancyvrb}
\RecustomVerbatimCommand{\VerbatimInput}{VerbatimInput}{fontsize=\footnotesize,
 % breaklines=true,
 % breakanywhere=true, 
 %breaksymbol=,
 commandchars=\\\{\},
 frame=single,  
 framesep=0.5em, % separation between frame and text
 labelposition=topline,
}
\input{include}
\input{header}
% \usepackage{arydshln}
% %\usepackage{pifont}  % for checkmark and xmark
% %\usepackage[table,xcdraw]{xcolor}
% %\usepackage{graphicx} % required for \rotatebox
% \usepackage{amssymb}    % for arrows

\title{Expanding the Action Space of LLMs\\ to Reason Beyond Language}
% Learning Actions Beyond Vocab for LLMs to Reason with External Environments
% WANT: external environments

% Symbolizing Interactions with Environments as Expanded Action Space of LLMs
% Expanding the Action Space of LLMs to Interact with Environments
% beyond language?
% teaching/incentivizing LLM to use non-language to interact xxx
% symbolic?
% LLMs? LLM? or full name
% <tool_call>calculator(579*8934)</tool_call>
% <results>xxx</results>
% fdsafsd calculate
% D*50000
% D*(150k+150k)
% <calculator> 43243 * </calculator> <result> Syntax error </result>
% calculate 12314*4314=4525252

% Authors must not appear in the submitted version. They should be hidden
% as long as the \iclrfinalcopy macro remains commented out below.
% Non-anonymous submissions will be rejected without review.

\author{Antiquus S.~Hippocampus, Natalia Cerebro \& Amelie P. Amygdale \thanks{ Use footnote for providing further information
about author (webpage, alternative address)---\emph{not} for acknowledging
funding agencies.  Funding acknowledgements go at the end of the paper.} \\
Department of Computer Science\\
Cranberry-Lemon University\\
Pittsburgh, PA 15213, USA \\
\texttt{\{hippo,brain,jen\}@cs.cranberry-lemon.edu} \\
\And
Ji Q. Ren \& Yevgeny LeNet \\
Department of Computational Neuroscience \\
University of the Witwatersrand \\
Joburg, South Africa \\
\texttt{\{robot,net\}@wits.ac.za} \\
\AND
Coauthor \\
Affiliation \\
Address \\
\texttt{email}
}

% The \author macro works with any number of authors. There are two commands
% used to separate the names and addresses of multiple authors: \And and \AND.
%
% Using \And between authors leaves it to \LaTeX{} to determine where to break
% the lines. Using \AND forces a linebreak at that point. So, if \LaTeX{}
% puts 3 of 4 authors names on the first line, and the last on the second
% line, try using \AND instead of \And before the third author name.

%\iclrfinalcopy % Uncomment for camera-ready version, but NOT for submission.
\begin{document}

\input{sections/z_app}

\bibliography{iclr2026_conference}
\bibliographystyle{iclr2026_conference}
\end{document}
